# Supplementary material for: Atomistic structure search using local surrogate mode
Source: arXiv:2208.09273 source file (2022-08-19)
Supplement: Supplementary file 1 [file supplementary-material.pdf]

# Supplementary material: Atomistic structure search using local surrogate model

Nikolaj Rønne,[1] Mads-Peter V. Christiansen,[1] Andreas Møller Slavensky,[1] Zeyuan Tang,[1] Florian Brix,[1] Mikkel Elkjær Pedersen,[1] Malthe Kjær Bisbo,[1] and Bjørk Hammer[1, a)]
*Center for Interstellar Catalysis, Department of Physics and Astronomy, Aarhus University, DK-8000 Aarhus, Denmark*

## I. DFT SETTING

All DFT evaluations except $CoB_{18}^-$ are performed using GPAW.[1,2] All DFT evaluations use the Perdew-Burke-Ernzerhof functional.[3] Below are the specific settings for each systems.

$C_5NH_5$: PBE functional in LCAO mode using dzp basis set and $(1,1,1)$ $k$-points.

$C_{30}$: PBE functional in LCAO mode using dzp basis set and $(1,1,1)$ $k$-points.

$Ti_{13}$: PBE functional in plane-wave mode with a cutoff of 400eV using $(1,1,1)$ $k$-points and a four-electron Ti setup.

$B_{12}$: PBE functional in plane-wave mode with a cutoff of 500eV using $(2,2,2)$ $k$-points with periodic boundary conditions.

$Ag_{12}S_6$: PBE functional in LCAO mode using dzp basis set and $(1,1,1)$ $k$-points.

$(MgSO_3)_4$: PBE functional in LCAO mode using dzp basis set and $(1,1,1)$ $k$-points.

$Cu_{10}$ on $ZnO(10\bar{1}0)$: PBE functional in plane-wave mode with a cutoff of 300eV and $(1,1,1)$ $k$-points with periodic boundary conditions.

$Ag_XO_Y$: PBE functional in LCAO mode using dzp basis set and $(3,3,1)$ $k$-points with periodic boundary conditions.

The $CoB_{18}^-$ DFT evaluations are performed with the ORCA code with the following settings.[4]

$CoB_{18}^-$: PBE functional using the def2-SVP basis set and a charge setting of $-1$ and multiplicity of 1.

## II. SOAP SETTINGS

SOAP settings as implemented in the DScribe package.[5] All descriptors use a polynomial weighing function with $r_0 = r_{\mathrm{cut}}$, $m = 2$ and $c = 1$.

| System | $n_{\mathrm{max}}$ | $l_{\mathrm{max}}$ | $\sigma$ | $r_{\mathrm{cut}}$ |
|---|---|---|---|---|
| $C_5NH_5$ local | 3 | 2 | 1.0 | 3.0 |
| $C_5NH_5$ global | 3 | 2 | 0.5 | 4.0 |
| $C_{30}$ | 4 | 3 | 0.75 | 4.0 |
| $Ti_{13}$ | 3 | 2 | 0.5 | 4.5 |
| $B_{12}$ | 4 | 3 | 1.0 | 4.0 |
| $CoB_{18}^-$ | 4 | 3 | 0.5 | 5.0 |
| $Ag_{12}S_6$ | 3 | 2 | 0.5 | 4.5 |
| $(MgSO_3)_4$ | 3 | 2 | 1.0 | 4.0 |
| $Cu_{10}$ on $ZnO(10\bar{1}0)$ | 3 | 2 | 1.0 | 5.0 |
| $Ag_XO_Y$ | 3 | 2 | 1.0 | 5.0 |

## III. SEARCH SETTINGS

The temperature for worker with index $i$ is calculated as

$$T_i = T_{\mathrm{min}} x^i, \tag{1}$$

where $T_{\mathrm{min}}$ and $x$ are search hyperparameters. Below are the search details for each system. The steps are the number of DFT local relaxations steps performed per iteration.

| System | $N_{\mathrm{workers}}$ | $T_{\mathrm{min}}$ [K] | $x$ | steps [#] |
|---|---|---|---|---|
| $C_5NH_5$ | 4 | 0.05 | 1.5 | 1 |
| $C_{30}$ | 4 | 0.05 | 3.0 | 1 |
| $Ti_{13}$ | 4 | 0.05 | 3.0 | 1 |
| $B_{12}$ | 4 | 0.05 | 3.0 | 1 |
| $CoB_{18}^-$ | 10 | 0.05 | 1.5 | 10 |
| $Ag_{12}S_6$ | 4 | 0.1 | 1.5 | 2 |
| $(MgSO_3)_4$ | 4 | 0.125 | 2.0 | 3 |
| $Cu_{10}$ on $ZnO(10\bar{1}0)$ | 4 | 0.05 | 4.18 | 1 |

The structural search for $Cu_{10}$ on $ZnO(10\bar{1}0)$ was performed in a confining box of size $9.16 \times 4.6 \times 4$ Å. Relieving this search constraint does lead to the finding of other, more stable structures than the one shown.

The $Ag_XO_Y$ concurrent multi-stoichiometry search is performed using twelve workers with different stoichiometries, a temperature of 3.0 eV and performing one DFT local relaxation step per iteration.

## IV. REFERENCES

[1] J. J. Mortensen, L. B. Hansen, and K. W. Jacobsen, Phys. Rev. B **71**, 035109 (2005).
[2] J. Enkovaara, C. Rostgaard, J. J. Mortensen, J. Chen, M. Dułak, L. Ferrighi, J. Gavnholt, C. Glinsvad, V. Haikola, H. A. Hansen,

a) Electronic mail: hammer@phys.au.dk

H. H. Kristoffersen, M. Kuisma, A. H. Larsen, L. Lehtovaara, M. Ljungberg, O. Lopez-Acevedo, P. G. Moses, J. Ojanen, T. Olsen, V. Petzold, N. A. Romero, J. Stausholm-Møller, M. Strange, G. A. Tritsaris, M. Vanin, M. Walter, B. Hammer, H. Häkkinen, G. K. H. Madsen, R. M. Nieminen, J. K. Nørskov, M. Puska, T. T. Rantala, J. Schiøtz, K. S. Thygesen, and K. W. Jacobsen, J. Phys. Condens. Matter **22**, 253202 (2010).

[3] J. P. Perdew, K. Burke, and M. Ernzerhof, Phys. Rev. Lett. **77**, 3865 (1996).

[4] F. Neese, Wiley Interdiscip. Rev. Comput. Mol. Sci. **2**, 73 (2012).

[5] L. Himanen, M. O. J. Jäger, E. V. Morooka, F. Federici Canova, Y. S. Ranawat, D. Z. Gao, P. Rinke, and A. S. Foster, Comput. Phys. Commun. **247**, 106949 (2020).
